# Supplementary material for: Role of minimum adhesive wear particle size in third-body layer properties
Source: arXiv:2304.14783 source file (2023-07-27)
Supplement: Supplementary file 1 [file appendix.tex]

% \onecolumn
\small
\appendix

\setcounter{figure}{0}
\setcounter{table}{0}
\setcounter{equation}{0}

\section{Appendix}
